# Supplementary material for: Incremental Sparse Bayesian Ordinal Regression
Source: arXiv:1806.06553 source file (2018-06-18)
Supplement: Supplementary file 1 [file supplement.tex]

%!TEX root = main.tex

\section*{Appendix}

In this section, we describe the derivation of fast marginal learning in more precious words. 
We mainly consider the contribution of $\boldsymbol{\alpha}$ to the marginal likelihood, denoted by $p(\mathbf D\mid \boldsymbol \alpha)$, and write it as follows: 
\begin{equation}\label{eq:mlalpha}
\ln p(\mathbf D\mid \boldsymbol \alpha) = \mathcal{L}-\frac{1}{2}\ln|\mathbf{C}| - \frac{1}{2}\hat{t}\mathbf{C}^{-1}\hat{t},
\end{equation}
where $\mathbf{C}$ is computed as: 
\begin{equation}
\begin{split}
\mathbf{C} &= \mathbf{H}^{-1} + \boldsymbol{\Phi} \mathbf{A}^{-1}\Phi^T\\
&= \mathbf{H}^{-1} + \sum_{n\neq j}\alpha_n\boldsymbol \phi_n \boldsymbol \phi_n^T + \alpha_j^{-1}\boldsymbol\phi_j\boldsymbol\phi_j^T.
\end{split}
\label{eq:C}
\end{equation}
Since computing $\mathbf{C}$ requires matrix inversion, which is time consuming and not applicable for large scale data, we exploit fast marginal likelihood learning \cite{IRVM}, and decompose Equation~\ref{eq:mlalpha} as follows:
\begin{itemize}
	\item First, based on Equation~\ref{eq:C}, we compute the matrix determination and inverse of $\mathbf{C}$ as follows:
	\begin{equation}
	\begin{split}
	|\mathbf{C}| &= |\mathbf{C}_{/j}|| \mathbf{I} + \alpha_j^{-1}\boldsymbol{\phi}_j\boldsymbol{\phi}_j^T| \\
	\mathbf{C}^{-1} &= \mathbf{C}_{/j}^{-1} - \frac{\mathbf{C}_{/j}^{-1}\boldsymbol{\phi}_j\boldsymbol{\phi}_j^T\mathbf{C}_{/j}^{-1}}{\alpha_j + \boldsymbol{\phi}_j^T\mathbf{C}_{/j}^{-1}\boldsymbol{\phi}_j}, 
	\end{split}
	\label{eq:c_decompose}
	\end{equation} 
	where $\mathbf{I}$ is the identity matrix, and $\mathbf{C}_{/j}$ denotes $\mathbf{C}$ without the contribution of $j$th sample. 
	
	\item Then, we define two vectors: 
	\begin{equation}\label{eq:qs}
	s_j = \phi_j^TC_{/j}^{-1}\phi_j, ~q_j = \phi_j^TC_{/j}^{-1}\hat{t}.
	\end{equation}
	Combining (\ref{eq:mlalpha}), (\ref{eq:c_decompose}) and (\ref{eq:qs}), we compute the contribution of each sample to the marginal likelihood: 		
	\begin{equation}\label{eq:singleML}
	\ln p(\boldsymbol D\mid \alpha_j) = \frac{1}{2}[\ln \alpha_j - \ln |\alpha_j + s_j| + \frac{q_j^2}{s_j+\alpha_j}]
	\end{equation}
	
	\item However, we still need matrix inversion in~\eqref{eq:qs}. In order to speed up the computation, we define the follow auxiliary variables: 
	\begin{eqnarray*}
	\begin{split}
	Q_j =&\boldsymbol{ \phi}_j^T \mathbf{C}^{-1}\hat{t}  =\boldsymbol{ \phi}_j^T \mathbf{H} \hat{t} - \boldsymbol{\phi}_j^T \mathbf{H} \boldsymbol{\Phi} \boldsymbol{\Sigma} \boldsymbol{\Phi}^T \mathbf{H} \hat{t} \\
	S_j = &\boldsymbol{ \phi}_j^T \mathbf{C}^{-1} \boldsymbol{\phi}_j = \boldsymbol{\phi}_j^T \mathbf{H} \boldsymbol{\phi}_j - \boldsymbol{\phi}_j^T \mathbf{H} \boldsymbol{\Phi} \boldsymbol{\Sigma} \boldsymbol{\Phi}^T \mathbf{H} \boldsymbol{\phi}_j. 
	\end{split}
	\label{eq:QS}
	\end{eqnarray*}
	Then we can compute $	s_j = \frac{\alpha_jS_j}{\alpha_j - S_j}$ and $q_j = \frac{\alpha_j Q_j}{\alpha_j-S_j}$.
	
	\item Finally, setting $\frac{\partial \ln p(\boldsymbol D\mid \boldsymbol \alpha)}{\partial \alpha_j}  = 0$, we get the closed form solution for $\alpha_j$:  
	\begin{equation}
	\alpha_j = \frac{s_j^2}{q_j^2-s_j}. \label{eq:alpha}  
	\end{equation}
	Since  $\alpha_j\geq0$, the denominator of Equation~\ref{eq:alpha}, $f_j = q_j^2-s_j $, should also be bigger than $0$, which works as an important criterion for determining the relevant samples.	
\end{itemize}

\noindent%
For the noise term $\sigma$, setting the derivative 
$\frac{\ln p(\mathbf{D}\mid \boldsymbol \eta)}{\sigma} = 0$, we obtain an update rule for the noise term: 
\begin{equation}
\sigma^2 = \frac{||\mathbf{\hat{t}}- \boldsymbol{\Phi w}||^2}{N - \sum_{n}(1-\alpha_n \Sigma_{nn})},
\label{eq:noise}
\end{equation}
where $\mathbf{\hat{t}} = \mathbf{H}^{-1} \boldsymbol{\delta} + \boldsymbol{\Phi}\mathbf{w}^*$ is defined as at the end of Section~\ref{sec:SBL:MAP}.
